# Supplementary material for: STFT Phase Retrieval: Uniqueness Guarantees and Recovery Algorithms
Source: arXiv:1508.02820 source file (2016-04-01)
Supplement: Supplementary file 1 [file AppendixB.tex]

\section{Alternative Proof of Theorem \ref{l1thm}}

\label{appB}

The affine constraints in (\ref{STFTPRR}) can be rewritten as (see Section \ref{appD}):
\begin{align}
\nonumber & a_w[ m , r ] = { \sum_{n = 0}^{N-1-m} X[n,n+m] w[ rL - n ]w^\star[rL-(n+m)] } \nonumber
\end{align}
Due the constraint corresponding to $r=0$, $\X$ has to satisfy:
\begin{equation}
\abs{w[0]}^2X[0,0] = {a_w[0,0]} = \abs{w[0]}^2\abs{x_0[0]}^2, \nonumber
\end{equation}
because of which $X[0,0]$ is fixed to $|x_0[0]|^2$ as $w[0] \neq 0$. Due to the constraints corresponding to $r=1$, $\X$ has to satisfy:
\begin{align}
& \abs{w[0]}^2X[1,1] + \abs{w[1]}^2X[0,0] = a_w[0,1] \nonumber \\
& \quad \quad \quad \quad = \abs{w[0]}^2\abs{x_0[1]}^2 + \abs{w[1]}^2\abs{x_0[0]}^2, \nonumber \\
& w^\star[0]w[1] X[0,1] = a_w[1,1] = w^\star[0]w[1]x_0[0]x_0^\star[1] \nonumber.
\end{align}
Since $X[0,0] =\abs{x_0[0]}^2$ and $w[0]w[1] \neq 0$, $X[1,1]$ and $X[0,1]$ are fixed to $|x_0[1]|^2$ and $x_0[0]x_0^\star[1]$ respectively.

Applying this argument incrementally, the measurements corresponding to short-time section $r$, with the help of the entries of $\X$ uniquely determined, fix the value of $X[r,r]$ and $X[r-1,r]$ to $\abs{x_0[r]}^2$ and  $x_0[r-1]x_0^\star[r]$ respectively. Hence, the diagonal and the first off-diagonal entries of every feasible matrix of (\ref{STFTPRR}) match the diagonal and the first off-diagonal entries of the matrix $\x_0\x_0^\star$. Since the entries are sampled from a rank one matrix with non-zero diagonal entries (i.e., $\x_0\x_0^\star$), there is exactly one positive semidefinite completion, which is the rank one completion $\x_0\x_0^\star$ \cite{horn}. 

In particular, due to the aforementioned determined entries of $\X$ and the positive semidefinite constraint $\X \succcurlyeq 0$, the convex program (\ref{STFTPRR}) has only one feasible matrix, given by $\x_0\x_0^\star$. The underlying signal $\x_0$ can be recovered (up to a global phase)  by a simple decomposition.
